# Supplementary material for: Optimizing Mentor-Student Communication with Symbolic Design for Message States
Source: arXiv:2312.04227 source file (2023-12-07)
Supplement: Supplementary file 1 [file 6_supplementary.tex]

\section{Supplementary Material}

% 预调研用户背景

% 问卷的用户背景
